# Supplementary material for: Community Detection in Networks with Node Attributes
Source: arXiv:1401.7267 source file (2014-01-28)
Supplement: Supplementary file 1 [file 070appendix.tex]

\begin{itemize}
	\item ...
\end{itemize}
